# Supplementary material for: PiXi: Password Inspiration by Exploring Information
Source: arXiv:2304.10728 source file (2023-09-28)
Supplement: Supplementary file 1 [file consentForm.pdf]

## **Consent Form to Participate in a Research Study**

**Title of Research Study:** A Study of Online Account Registration Methods

### **Introduction:**

You are invited to participate in a research study entitled *A study of online account registration methods*. Please read the information about the study presented in this form. The form includes details on study's procedures, risks, and benefits that you should know before you decide if you would like to take part. You should take as much time as you need to make your decision. You should ask the Principal Investigator (PI) or study team to explain anything that you do not understand and make sure that all of your questions have been answered before agreeing to this consent form. Before you make your decision, feel free to talk about this study with anyone you wish, including your friends and family. Participation in this study is voluntary. This study has been reviewed by the University of Ontario Institute of Technology (Ontario Tech University) Research Ethics Board [insert REB assigned #] on [insert date].

### **Purpose and Procedure:**

#### **Purpose:**

This research aims to test whether a new user interface nudges users to choose secure and memorable passwords.

#### **Procedures:**

There are approx. 500-1500 participants in this study. The research activity and data storage are occurring in Canada.

This study has 2 sessions:

| <b>Session</b>                    | <b>Study procedure</b>                                                                                                                                                                                                                                                                  | <b>Duration of session</b> |
|-----------------------------------|-----------------------------------------------------------------------------------------------------------------------------------------------------------------------------------------------------------------------------------------------------------------------------------------|----------------------------|
| Session 1                         | <ol style="list-style-type: none"><li>1. Go to the register page, use our system to navigate through some book, movie, music, or image-related information (much like an internet search), and register an account. (2-3 mins)</li><li>2. Complete a questionnaire. (2-4mins)</li></ol> | 4-7 mins                   |
| Session 2, 7 days after Session 1 | <ol style="list-style-type: none"><li>1. Go to the login page and login. (0 - 1min)</li><li>2. Complete a questionnaire. (0 - 1 min)</li></ol>                                                                                                                                          | 1-2 mins                   |

Please ensure that you answer the questionnaires on your own without any assistance from others. We would kindly ask you to take your time to carefully consider your answers for each of the questions.

### **Potential Benefits:**

Aside from receiving compensation, you will not directly benefit from participating in this study. Your participation will contribute to knowledge about nudging in password systems, which may help researchers design more secure and memorable password approaches.

### **Potential Risks or Discomforts:**

The greatest potential risk is a breach of the data we collect. Although we employ best practices for security and ensure your information will be stored with an anonymous identifier, we ask that you please do not use your existing passwords in this research study or reuse any passwords created in this study.

Our system will ask you to search and navigate through some book, movie, music, or image-related information, much like an internet search. It is unlikely, but possible, that some images or words shown by the system may contain visual or verbally offensive and/or inappropriate information (e.g., covers for horror movies or violent images).

### **Use and Storage of Data:**

The data includes demographic information and feedback (i.e., gender, age, and education level). All the data is anonymous, and the data doesn't include any personal, confidential, or valuable information.

### **Confidentiality:**

Your MTurk ID will be kept confidential. Collected data will be anonymous and it will not include any information that reveals your identity. Your privacy shall be respected. No information about your identity will be shared or published without your permission, unless required by law. Confidentiality will be provided to the fullest extent possible by law, professional practice, and ethical codes of conduct. Please note that confidentiality cannot be guaranteed while data is in transit over the Internet.

This research study includes the collection of demographic data which will be aggregated in an effort to protect your anonymity. Despite best efforts it is possible that your identity can be determined even when data is aggregated.

### **Voluntary Participation:**

Your participation in this study is voluntary and you may partake in only those parts of the study in which you feel comfortable. You may also decide not to be in this study, or to be in the study now, and then change your mind later.

You may refuse to answer any question you do not want to answer, or not answer an interview question by saying, 'preferred not to answer'.

### **Right to Withdraw:**

You can withdraw at any time simply by leaving our website and not submitting your data. If you withdraw from the research project prior to submitting your data at the end of a session, any data collected in that session will be removed. If you wish to withdraw after completing a session, you can do so within one week by contacting the researchers directly by email. You do not need to offer any reason for your withdrawal.

### **Compensation, Reimbursement, Incentives:**

You will be compensated \$0.85 for completing Session 1. Once you have submitted your data you will receive a completion code to enter on Amazon MTurk. Once you begin the Session 1 questionnaire, which is about 50% of the way through Session 1, you may choose to withdraw by clicking a withdraw button. If you click this button on any page of the questionnaire, you will receive a 50% completion code to enter on MTurk, which will provide you \$0.42 (approx. 50% of the Session 1 compensation). If you complete Session 1, you will be invited to participate in Session 2 through Amazon MTurk, for which you will be compensated \$0.35 USD after submitting your completion code to Amazon MTurk.

Once you begin the Session 2 questionnaire, which is about 50% of the way through Session 2, you may choose to withdraw by clicking a withdraw button. If you click this button on any page of the questionnaire, you will receive a 50% completion code to enter on MTurk, which will provide you \$0.18 (approx. 50% of the Session 2 compensation).

### **Debriefing and Dissemination of Results:**

After the study is complete, we will publish aggregated and anonymous data in a research paper. If you are interested in the study, please contact [shengqian.wang@ontariotechu.net](mailto:shengqian.wang@ontariotechu.net) to provide you with the results of the study after the research is published. .

### **Participant Rights and Concerns:**

Please read this consent form carefully and feel free to ask the researcher any questions that you might have about the study. If you have any questions about your rights as a participant in this study, complaints, or adverse events, please contact the Research Ethics Office at (905) 721-8668 ext. 3693 or at [researchethics@ontariotechu.ca](mailto:researchethics@ontariotechu.ca).

If you have any questions concerning the research study or experience any discomfort related to the study, please contact the researcher Shengqian Wang at [shengqian.wang@ontariotechu.net](mailto:shengqian.wang@ontariotechu.net).

By signing this form you do not give up any of your legal rights against the investigators, sponsor or involved institutions for compensation, nor does this form relieve the investigators, sponsor or involved institutions of their legal and professional responsibilities.

**Secondary Use of Research for Future Research Purposes:**

Please note, if you agree to participate (and do not withdraw from the study), your anonymous data may also be used for future research studies relating to our research on password authentication systems, etc.

**Consent to Participate:**

1. *I have read the consent form and understand the study being described.*
2. *I have had an opportunity to ask questions and my questions have been answered. I am free to ask questions about the study in the future.*
3. *I freely consent to participate in the research study, understanding that I may discontinue participation at any time without penalty.*
4. *I understand the possible need for secondary research uses of my research data for future research use and provide consent for the use of my data to be used in future studies.*
5. *The study may contain graphic or textual content that may be inappropriate or offensive to some users.*
6. *Discretion while searching and exploring content on the system is advised.*

☐ **I agree**

☐ **I understand and wish to proceed**
