# Supplementary material for: PiXi: Password Inspiration by Exploring Information
Source: arXiv:2304.10728 source file (2023-09-28)
Supplement: Supplementary file 2 [file questionnaire1.pdf]

# Session 1 questionnaire

## Basic Information

- A. Area of Work
  - a. Architecture and engineering
  - b. Arts, culture and entertainment
  - c. Business, management and administration
  - d. Communications
  - e. Community and social services
  - f. Education
  - g. Science and technology
  - h. Installation, repair and maintenance
  - i. Farming, fishing and forestry
  - j. Government
  - k. Health and medicine
  - l. Law and public policy
  - m. Sales
  - n. Prefer not to answer
- B. Level of Education
  - a. None, or less than secondary (high school)
  - b. Secondary diploma (high school graduation)
  - c. Bachelor's degree (three or more year program at a university, college, trade or technical school, or other institute)
  - d. Master's degree, or professional degree
  - e. Doctoral level university degree (PhD)
  - f. Prefer not to answer
- C. Gender
  - a. Male
  - b. Female
  - c. Prefer not to answer
- D. Language
  - a. English
  - b. Other
  - c. Prefer not to answer
- E. Age Range
  - a. Under 20
  - b. 20-30
  - c. 30-40
  - d. 40-50
  - e. 50-60
  - f. Above 60
  - g. Prefer not to answer

## Questionnaire

1. I'm reusing passwords for my accounts (not including this system).

1 (strongly disagree)    2 (disagree)    3 (neutral)    4 (agree)    5 (strongly agree)

6. (Prefer not to answer)

2. I'm using password manager(s) to help me manage passwords.

1 (strongly disagree)    2 (disagree)    3 (neutral)    4 (agree)    5 (strongly agree)

6. (Prefer not to answer)

3. I'm using random password generators to help me create passwords.

1 (strongly disagree)    2 (disagree)    3 (neutral)    4 (agree)    5 (strongly agree)

6. (Prefer not to answer)

4. Seven plus three = eight

1 (strongly disagree)    2 (disagree)    3 (neutral)    4 (agree)    5 (strongly agree)

6. (Prefer not to answer)

5. I believe this password creation method helped me to create a unique password.

1 (strongly disagree)    2 (disagree)    3 (neutral)    4 (agree)    5 (strongly agree)

6. (Prefer not to answer)

6. I would use this password creation method in this study frequently.

1 (strongly disagree)    2 (disagree)    3 (neutral)    4 (agree)    5 (strongly agree)

6. (Prefer not to answer)

7. The password creation method in this study is unnecessarily complex.

1 (strongly disagree)    2 (disagree)    3 (neutral)    4 (agree)    5 (strongly agree)

6. (Prefer not to answer)

8. The password creation method in this study was easy to use.

1 (strongly disagree)    2 (disagree)    3 (neutral)    4 (agree)    5 (strongly agree)

6. (Prefer not to answer)

9. I need the support of a technical person to be able to use the password creation method in this study.

1 (strongly disagree)    2 (disagree)    3 (neutral)    4 (agree)    5 (strongly agree)

6. (Prefer not to answer)

10. The various functions in this password creation method were well integrated.

1 (strongly disagree)    2 (disagree)    3 (neutral)    4 (agree)    5 (strongly agree)

6. (Prefer not to answer)

11. There was too much inconsistency in the password creation method in this study.

1 (strongly disagree)    2 (disagree)    3 (neutral)    4 (agree)    5 (strongly agree)

6. (Prefer not to answer)

12. Most people would learn to use the password creation method in this study very quickly.

1 (strongly disagree)    2 (disagree)    3 (neutral)    4 (agree)    5 (strongly agree)

6. (Prefer not to answer)

13. The password creation method in this study is very cumbersome to use.

1 (strongly disagree)    2 (disagree)    3 (neutral)    4 (agree)    5 (strongly agree)

6. (Prefer not to answer)

14. I felt very confident using the password creation method in this study.

1 (strongly disagree)    2 (disagree)    3 (neutral)    4 (agree)    5 (strongly agree)

6. (Prefer not to answer)

15. I needed to learn a lot of things before I could get going with the password creation method in this study.

1 (strongly disagree)    2 (disagree)    3 (neutral)    4 (agree)    5 (strongly agree)

6. (Prefer not to answer)
