# Supplementary material for: PiXi: Password Inspiration by Exploring Information
Source: arXiv:2304.10728 source file (2023-09-28)
Supplement: Supplementary file 3 [file addtionalAppendix.tex]

\section{PiXi \& PiXi-Hints APIs}
\begin{figure*}[h]
\centering
  \includegraphics[width=0.8\textwidth]{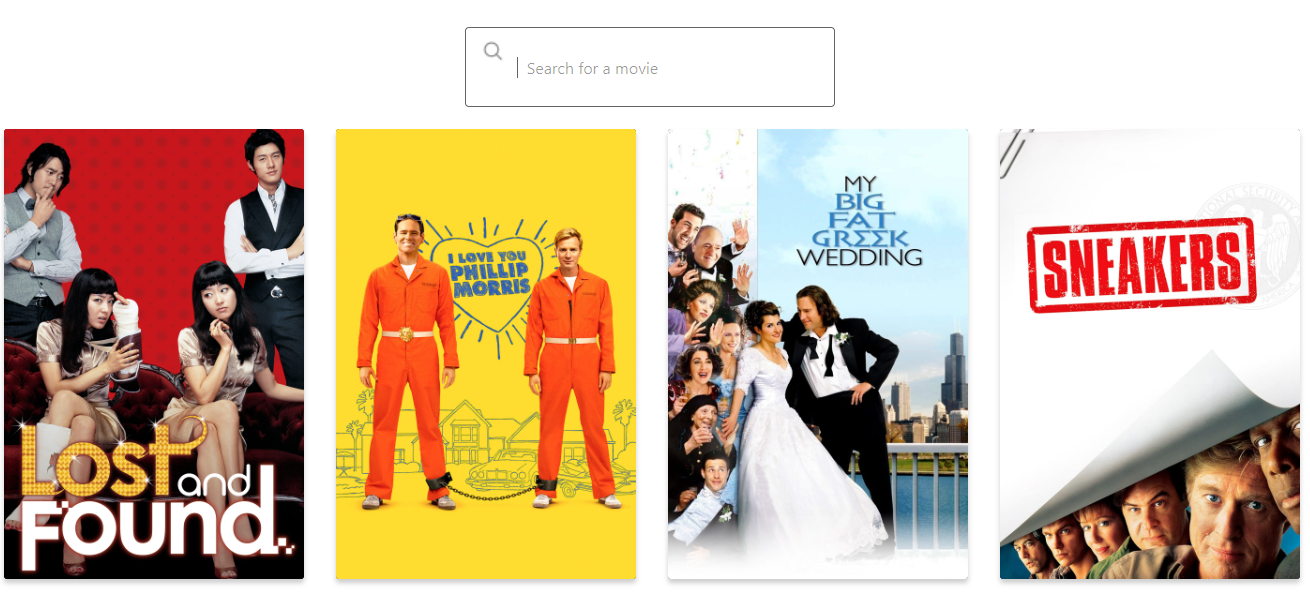} 
  \caption{The movie category page is using TMDB API. }
\end{figure*} 

\begin{figure*}[h]
\centering
  \includegraphics[width=0.8\textwidth]{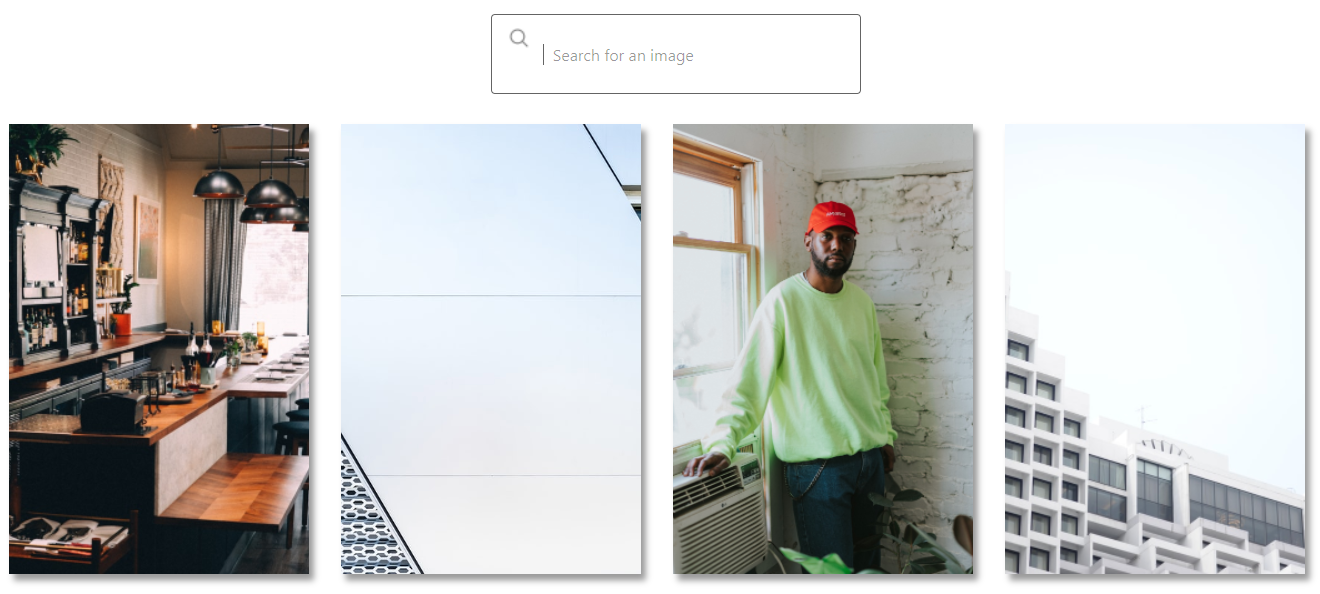} 
  \caption{The image category page is using Unplash API. }
\end{figure*} 

\begin{figure*}[h]
\centering
  \includegraphics[width=0.8\textwidth]{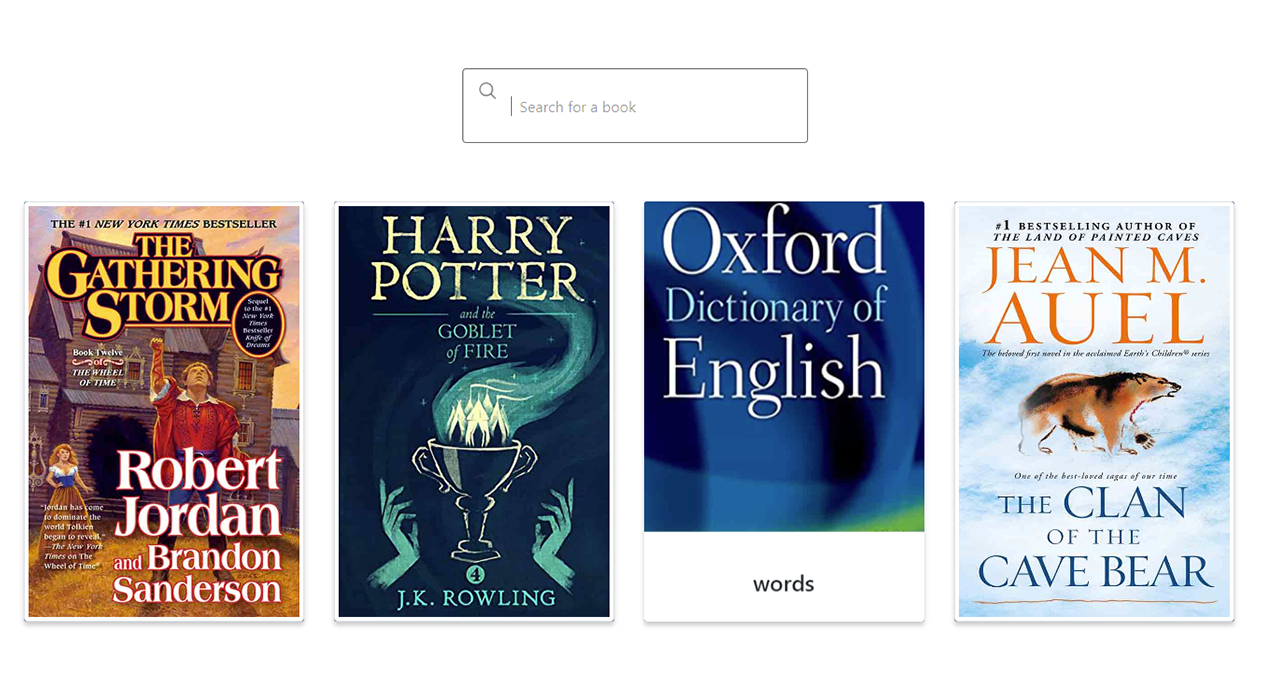} 
  \caption{The book category page is using an API made by the authors.}
\end{figure*}

\section{Mturk advertisement}
\setcounter{table}{0}
\section{Amazon MTurk Advertisement}
\begin{figure*}[h]
\centering
  \includegraphics[width=0.9\textwidth]{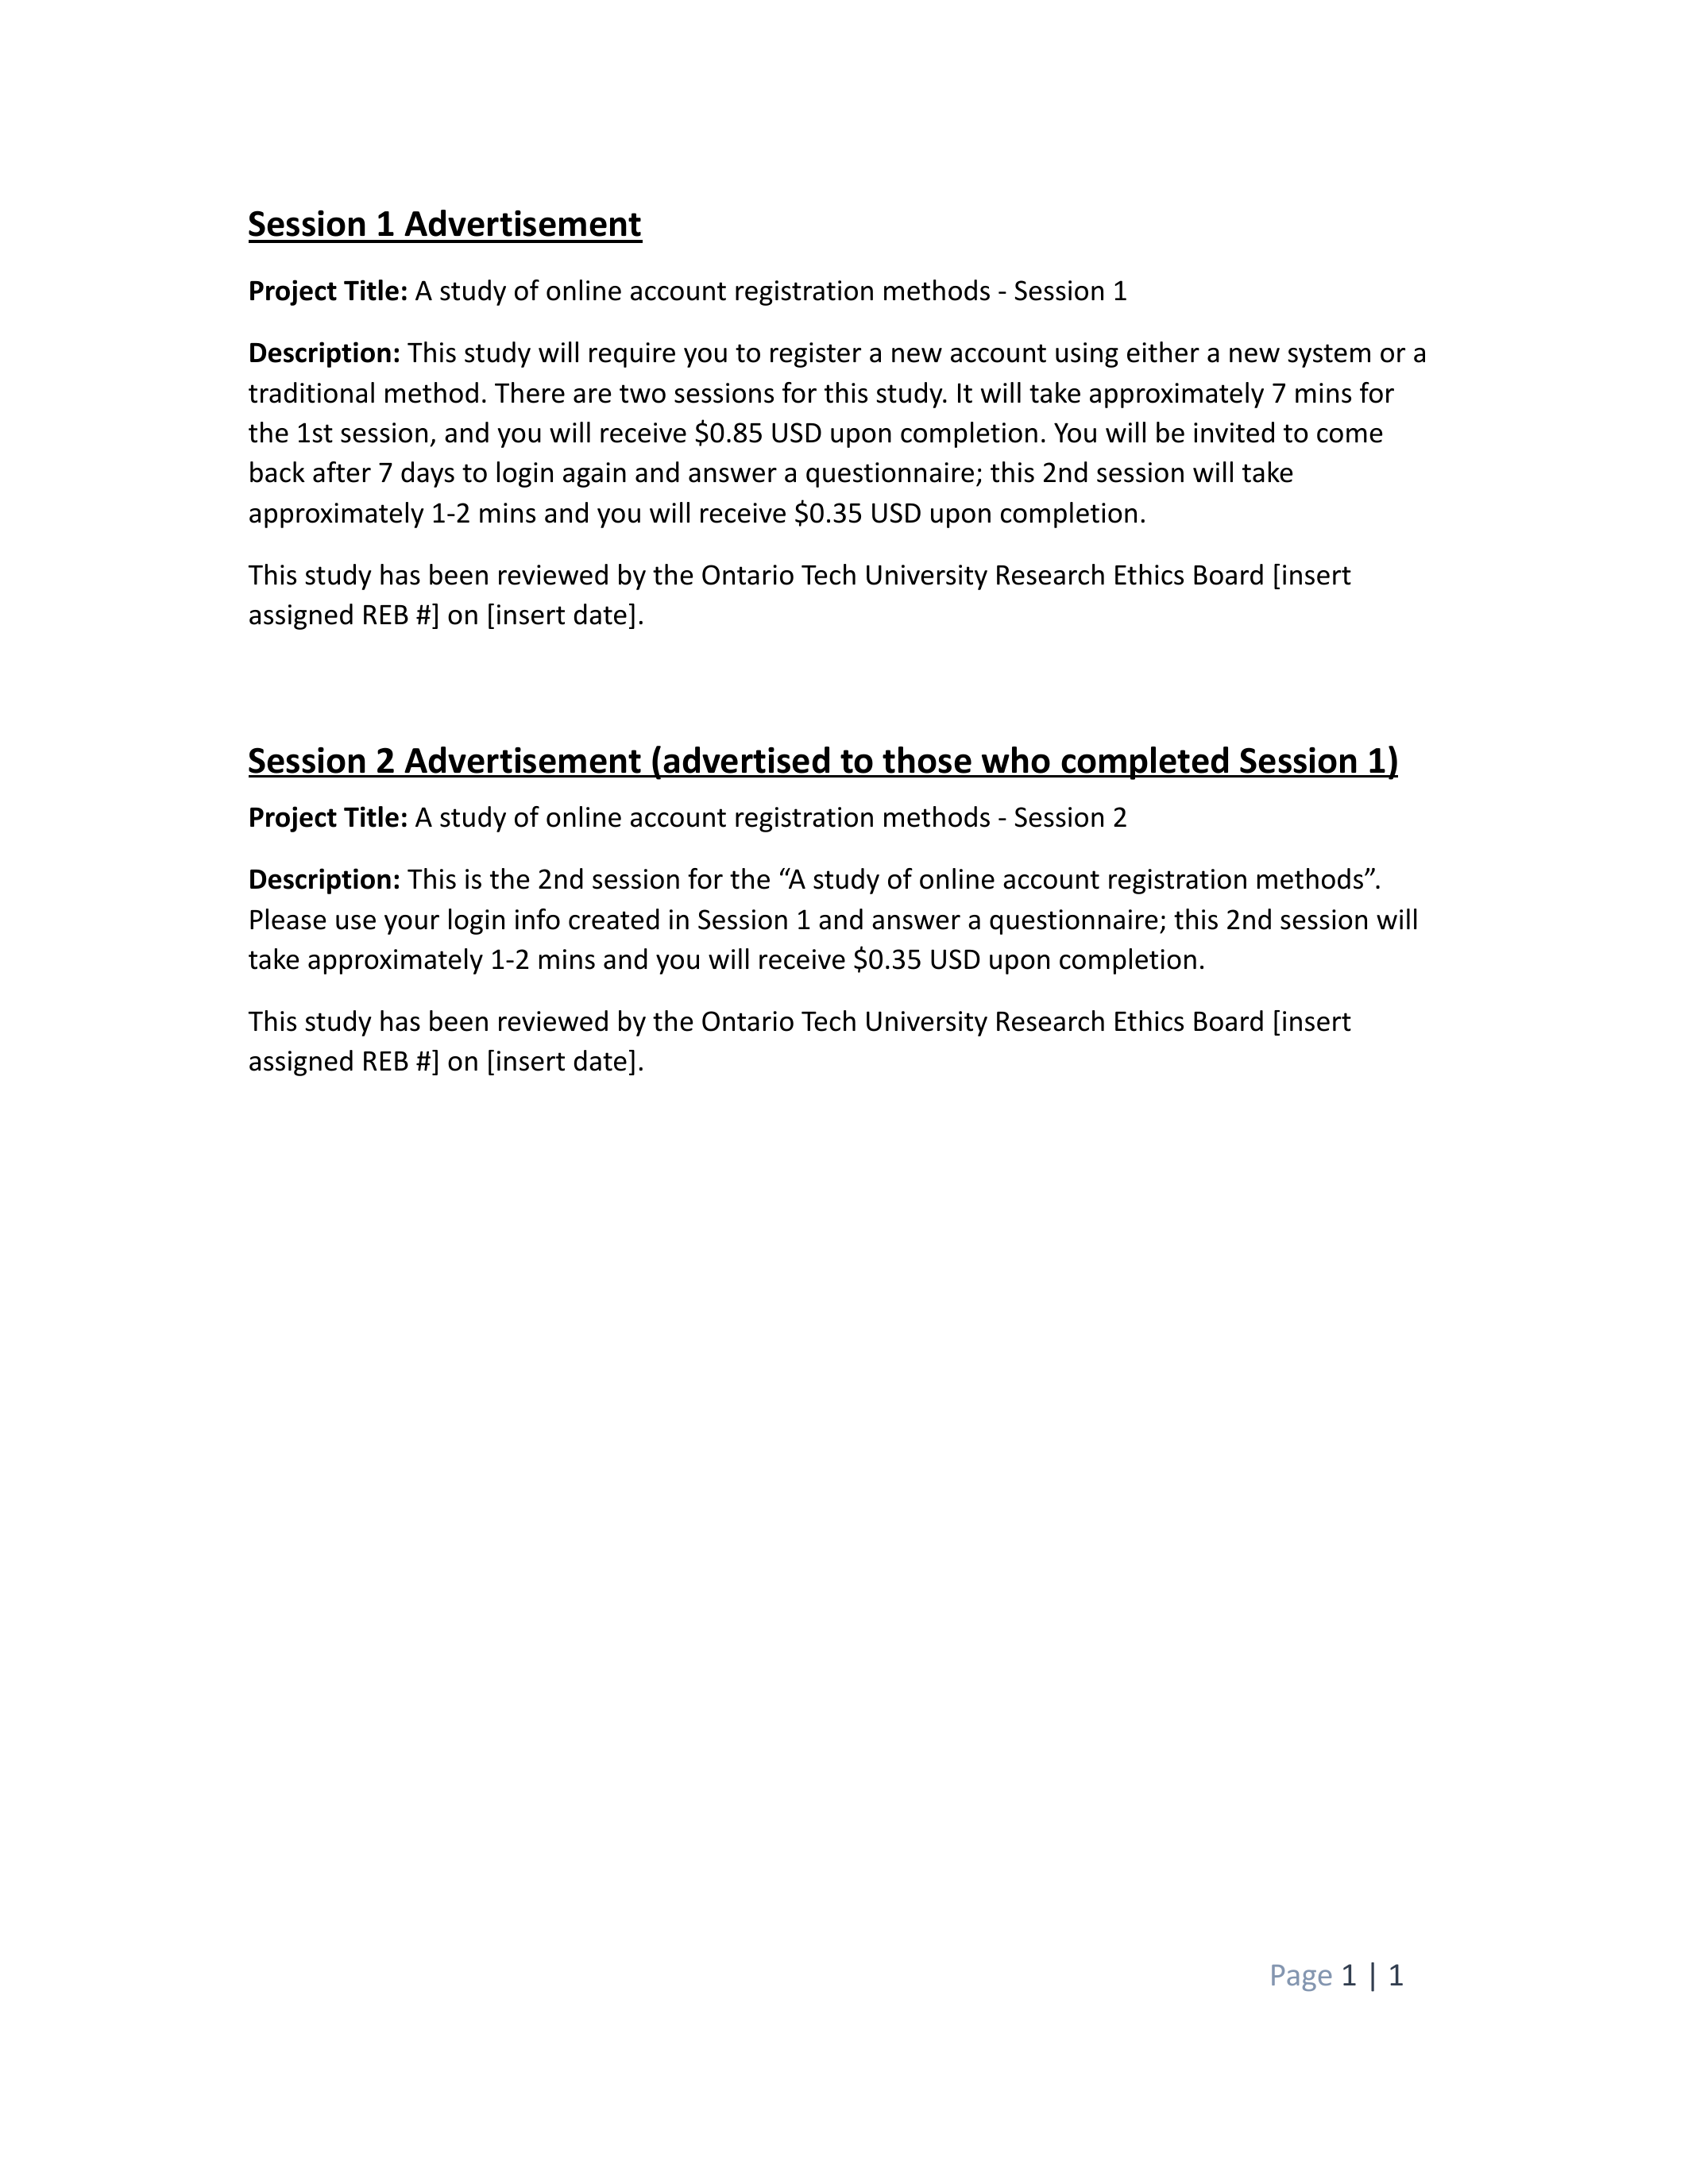} 
  \caption{Amazon MTurk Advertisement}
  \label{app:ad}
\end{figure*} 

\section{\label{app:consent}Appendix Consent Form}
\begin{figure*}[h]
\centering
  \includegraphics[width=0.8\textwidth,page=1]{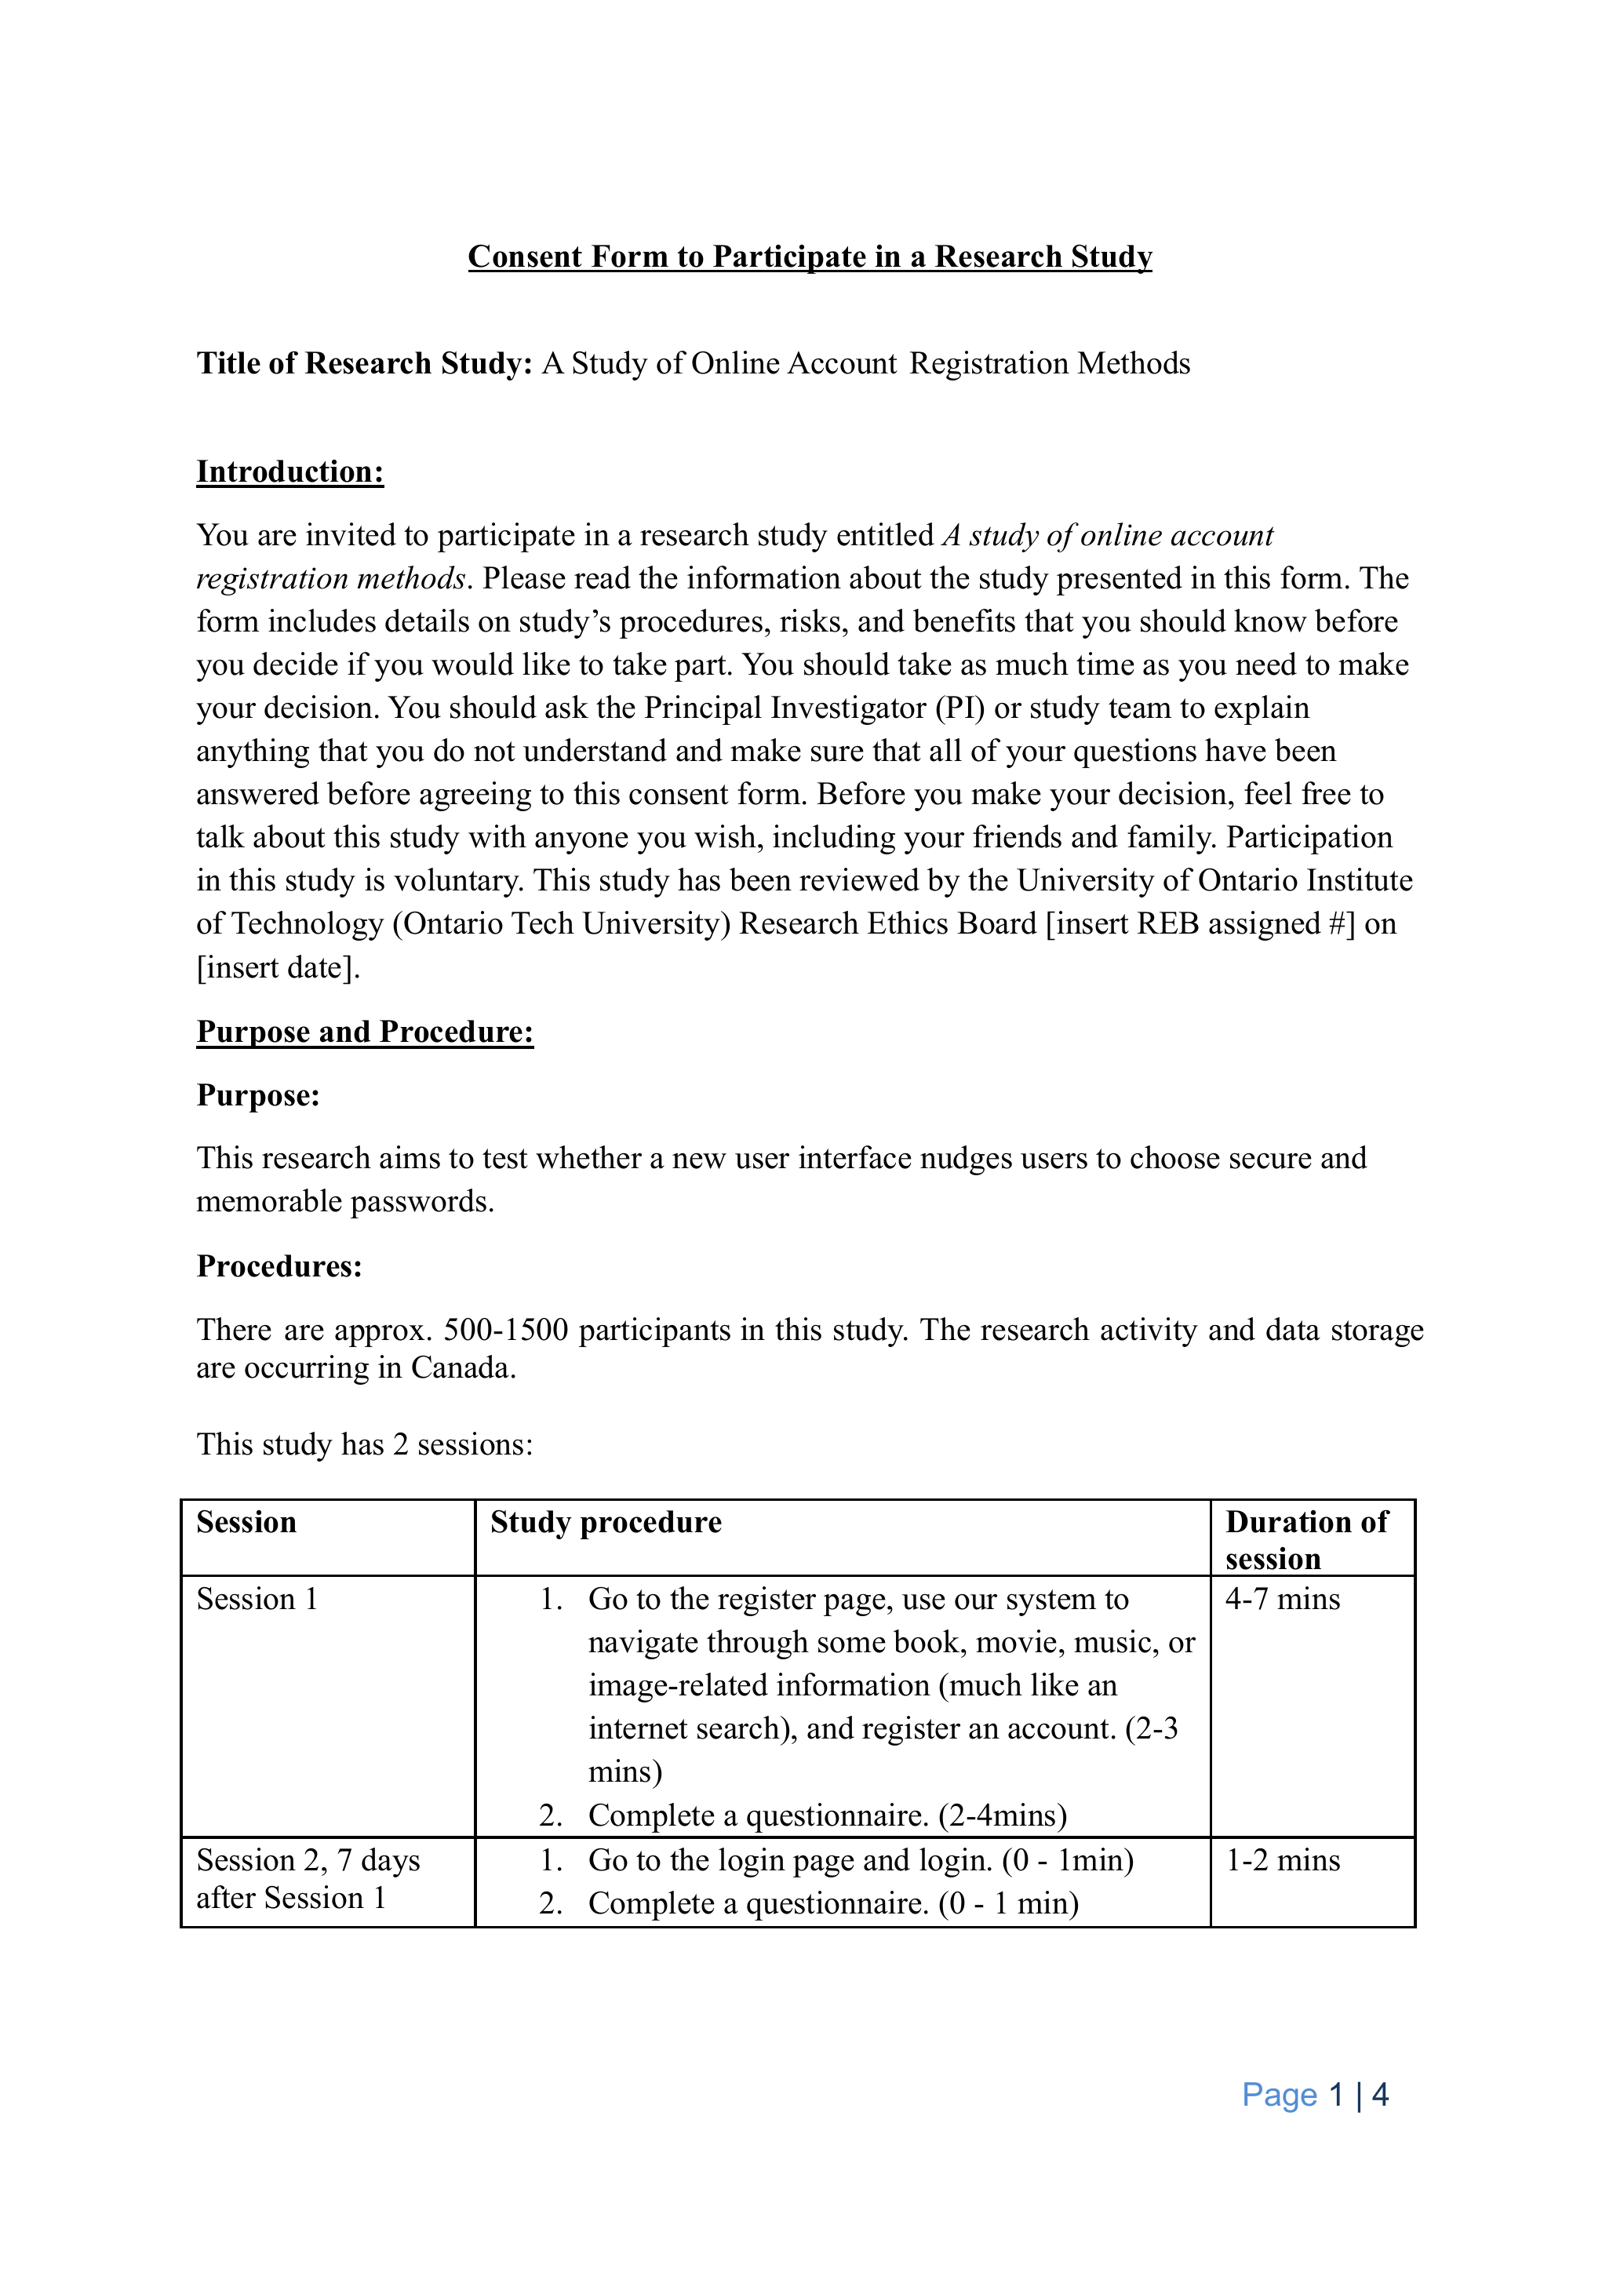} 
  \caption{Consent form, page 1/4}
\end{figure*} 
\begin{figure*}[h]
\centering
  \includegraphics[width=0.8\textwidth,page=2]{Appendix/consentForm.pdf} 
  \caption{Consent form, page 2/4}
\end{figure*}  
\begin{figure*}[h]
\centering
  \includegraphics[width=0.8\textwidth,page=3]{Appendix/consentForm.pdf} 
  \caption{Consent form, page 3/4}
\end{figure*}  
\begin{figure*}[h]
\centering
  \includegraphics[width=0.8\textwidth,page=4]{Appendix/consentForm.pdf} 
  \caption{Consent form, page 3/4}
\end{figure*}

\section{The book list}
\begin{table*}[b]
\centering
\begin{tabular}{ll|ll}
\hline
1  & The Gathering Storm - Chapter One               & 45 & SCleric Quintet 4 - The Fallen Fortress       \\ 
2  & 20,000 Leagues Under the Sea                    & 46 & Shadowdale                                    \\ 
3  & Alice in Wonderland                             & 47 & Spellfire                                     \\ 
4  & Beautiful and the Damned                        & 48 & Star Wars-Dark Force Rising                   \\ 
5  & Bible                                           & 49 & Star Wars-Heir to the Empire                  \\ 
6  & Breakfast at Tiffanys                           & 50 & Star Wars-The Last Command                    \\ 
7  & Clancy Tom - Patriot Games                      & 51 & Tantras                                       \\ 
8  & Clancy Tom - Red Storm Rising                   & 52 & Test Of The Twins                             \\ 
9  & Clarke Arthur C - 3001 The Final Odissey        & 53 & The Age Of Innocence                          \\ 
10 & Cleric Quintet 1 - Canticle                     & 54 & THE Catcher In The Rye                        \\ 
11 & Cleric Quintet 2 - In Sylvan Shadows            & 55 & The Fellowship Of The Ring                    \\ 
12 & Cleric Quintet 3 - Night Masks                  & 56 & The Great Gatsby                              \\ 
13 & Crown of Fire                                   & 57 & The Legend Of Huma                            \\ 
14 & Crucible - The Trial Of Cyric The Mad           & 58 & The little Prince                             \\ 
15 & Dragon lance Preludes 2 vol 2 - Flint the King  & 59 & The Lone Drow                                 \\ 
16 & Dragons of Autumn Twilight                      & 60 & The Return Of The King                        \\ 
17 & Dragons of Spring Dawning                       & 61 & The Second Generation                         \\ 
18 & Dragons of Summer Flame                         & 62 & The Thousand Orcs                             \\ 
19 & Dragons of Winter Night                         & 63 & The Two Swords                                \\ 
20 & Dragonwall                                      & 64 & The Two Towers                                \\ 
21 & Earth's Children 01 - The Clan of the Cave Bear & 65 & The Wheel of Time 01 - Eye of the world       \\ 
22 & Earth's Children 02 - The Valley of Horses      & 66 & The Wheel of Time 02 - The Great Hunt         \\ 
23 & Earth's Children 03 - The Mammoth Hunters       & 67 & The Wheel of Time 03 - The Dragon Reborn      \\ 
24 & Earth's Children 04 - Plains Of Passage         & 68 & The Wheel of Time 04 - The Shadow Rising      \\ 
25 & Earth's Children 05 - The Shelters Of Stone     & 69 & The Wheel of Time 05 - The Fires of Heaven    \\ 
26 & Frank Herbert - Children of Dune                & 70 & The Wheel of Time 06 - Lord of Chaos          \\ 
27 & Frank Herbert - Dune Messiah                    & 71 & The Wheel of Time 07 - A Crown of Swords      \\ 
28 & Frank Herbert - Dune                            & 72 & The Wheel of Time 08 - The Path of Daggers    \\ 
29 & Hamlet                                          & 73 & The Wheel of Time 09 - Winters Heart          \\ 
30 & Harry Potter 1 - Sorcerer's Stone               & 74 & The Wheel of Time 10 - Crossroads of Twilight \\ 
31 & Harry Potter 2 - Chamber of Secrets             & 75 & The Wheel of Time 11 - Knife of Dreams        \\ 
32 & Harry Potter 3 - The Prisoner Of Azkaban        & 76 & The Wheel of Time Prelude - New Spring        \\ 
33 & Harry Potter 4 - The Goblet Of Fire             & 77 & Time Of The Twins                             \\ 
34 & Harry Potter 5 - Order of the Phoenix           & 78 & To Kill a Mockingbird                         \\ 
35 & Harry Potter 6 - The Half Blood Prince          & 79 & The Tipping Point                             \\ 
36 & Harry Potter 7 - Deathly Hollows                & 80 & War Of The Twins                              \\ 
37 & Horselords                                      & 81 & Washington Square                             \\ 
38 & Maggie a girl of the streets                    & 82 & Waterdeep                                     \\ 
39 & Other half lives                                & 83 & {[}Chronicles Of Prydain 1{]} Book of Three   \\ 
40 & Pii                                             & 84 & {[}Chronicles Of Prydain 2{]} Black Cauldron  \\ 
41 & Pride and Prejudice                             & 85 & {[}Chronicles Of Prydain 3{]} Castle Of Llyr  \\ 
42 & Prince of Lies                                  & 86 & {[}Chronicles Of Prydain 4{]} Taran Wanderer  \\ 
43 & Robert Jordan - The Strike at Shayol Ghul       & 87 & {[}Chronicles Of Prydain 5{]} High King       \\ 
44 & Robinson Crusoe                                 &    &                                               \\ \hline
\end{tabular}
\caption{The book list of Books API.}
\label{tab:bookList}
\end{table*}

\section{PiXi Management System}
\begin{figure*}[h]
\centering
  \includegraphics[width=0.9\textwidth]{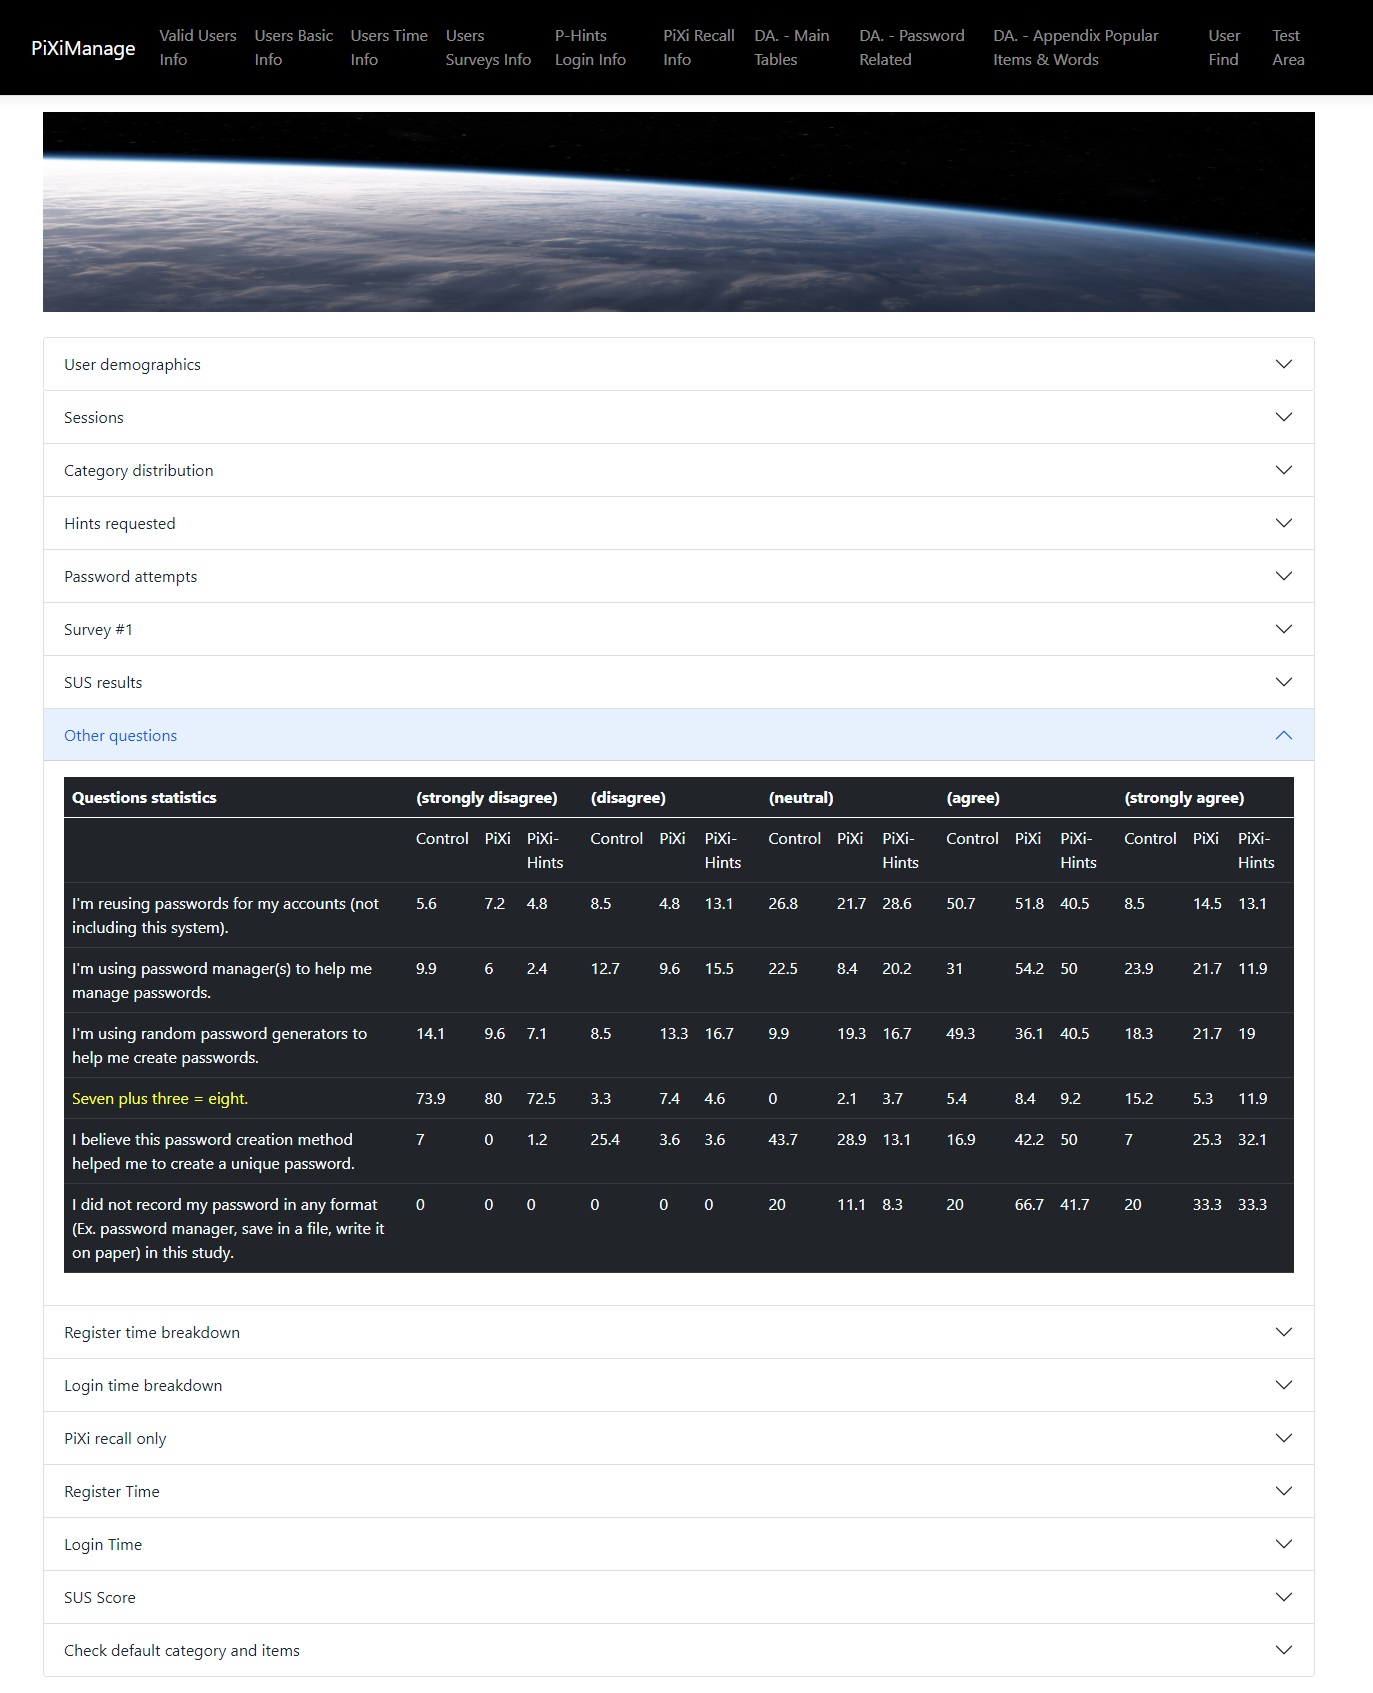} 
  \caption{PiXi Management System}
  \label{fig:PiXimanagement}
\label{pm} 
\end{figure*} 

\section{Appendix Session 1 - Questionnaire 1}
\begin{figure*}[h]
\centering
  \includegraphics[width=0.9\textwidth,page=1]{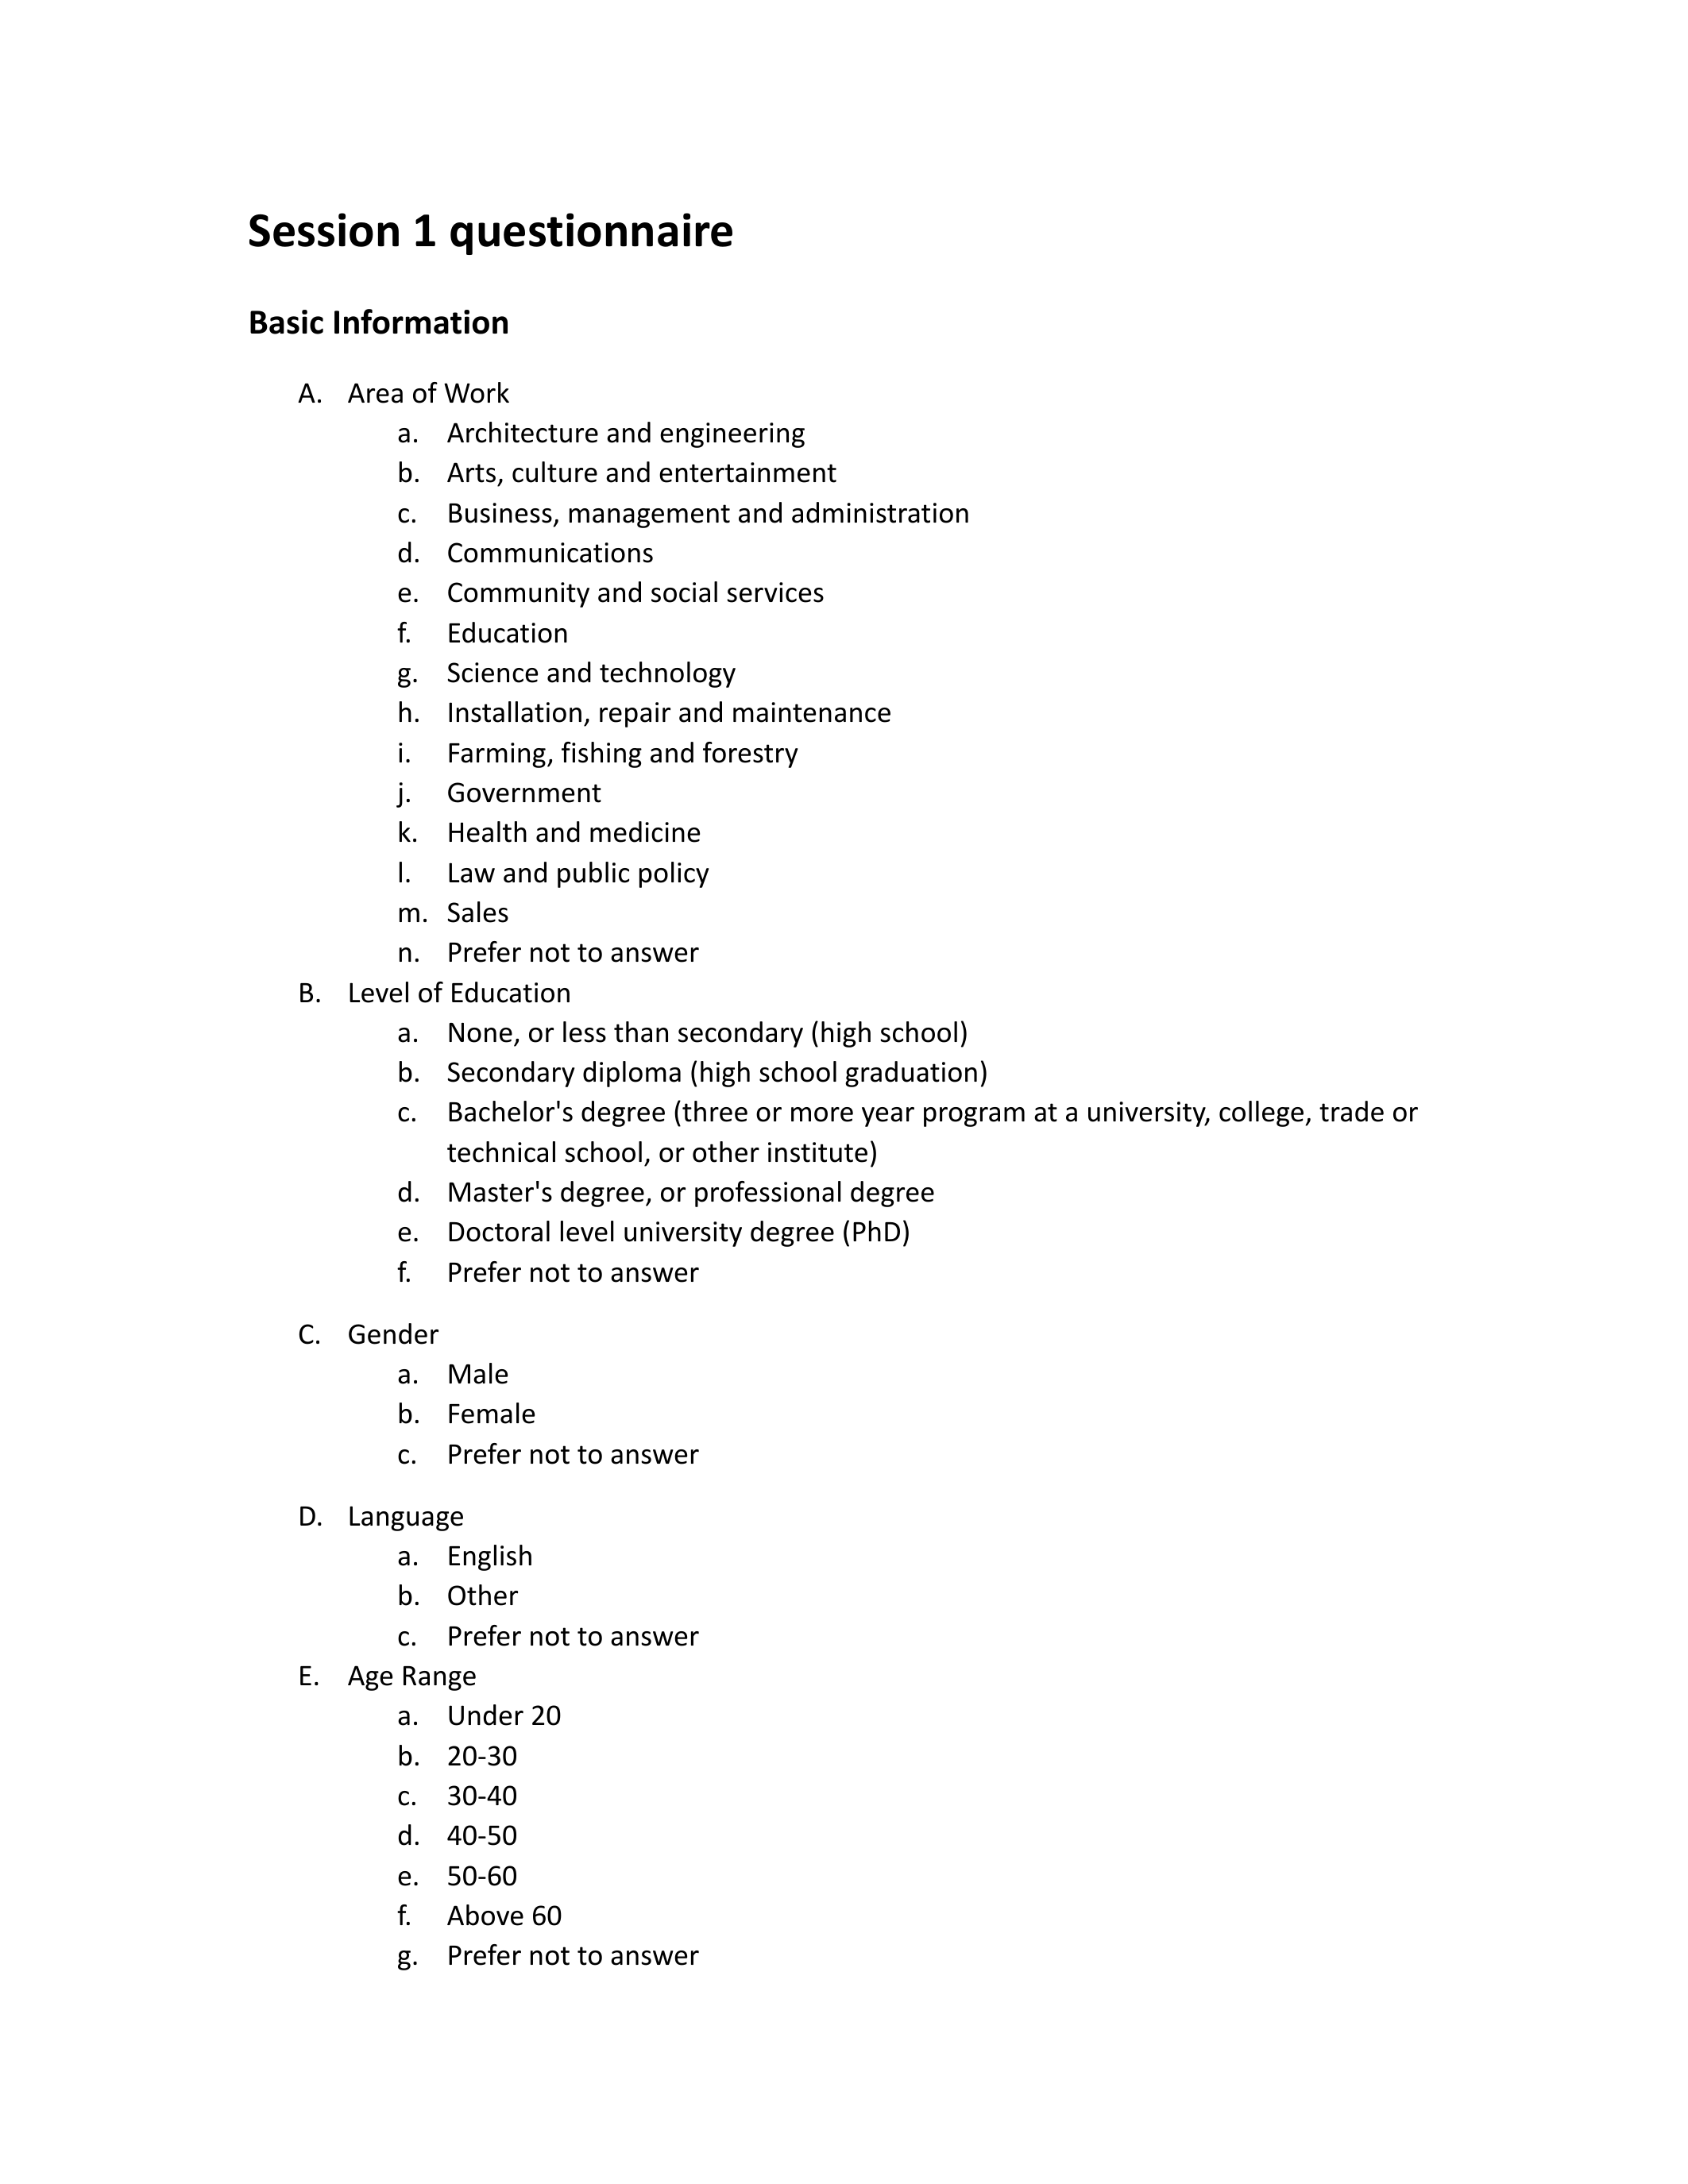} 
  \caption{Questionnaire 1, page 1/3.}
  \label{app:q1a}
\end{figure*} 

\begin{figure*}[h]
\centering
  \includegraphics[width=0.9\textwidth,page=2]{Appendix/questionnaire1.pdf} 
  \caption{Questionnaire 1, page 2/3.}
    \label{app:q1b}
\end{figure*} 

\begin{figure*}[h]
\centering
  \includegraphics[width=0.9\textwidth,page=3]{Appendix/questionnaire1.pdf} 
  \caption{Questionnaire 1, page 3/3.}
  \label{app:q1c}
\end{figure*} 

\section{Appendix Session 2 - Questionnaire 2}
\begin{figure*}[h]
\centering
  \includegraphics[width=0.9\textwidth]{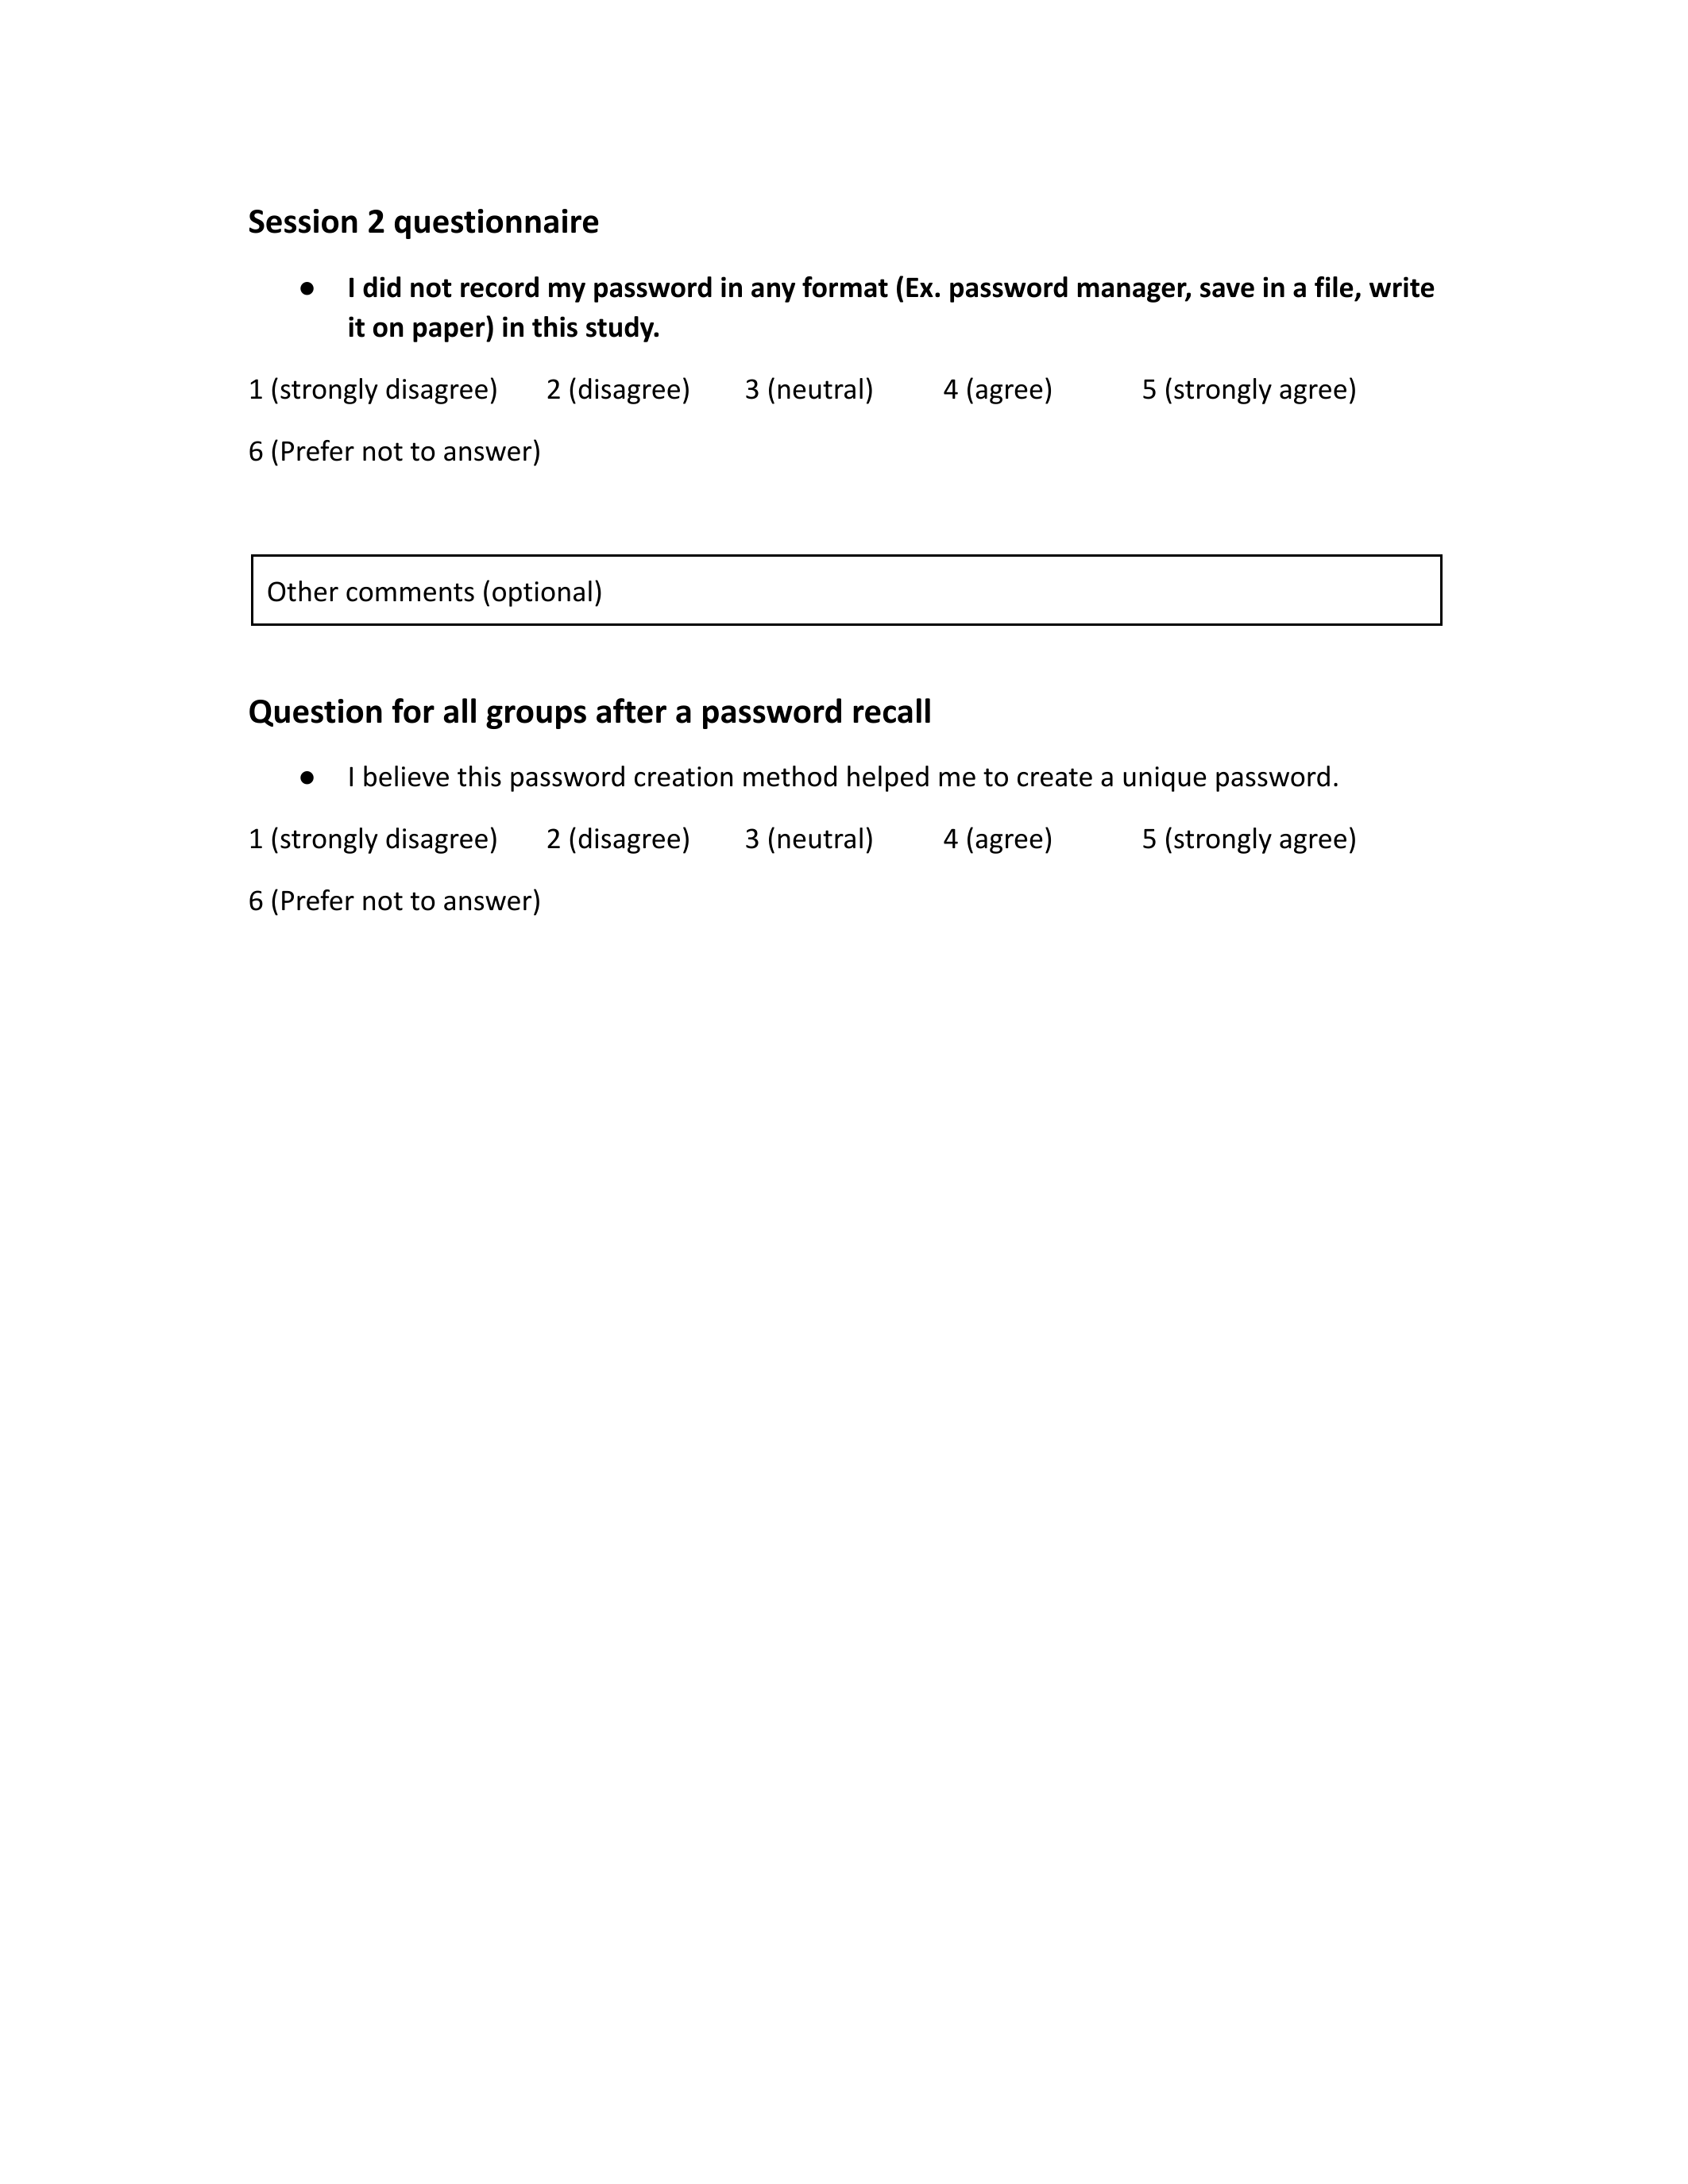} 
  \caption{Questionnaire 2, page 1/1.}
  \label{app:q2}
\end{figure*}
